# Supplementary material for: Typical entanglement for Gaussian states
Source: arXiv:1903.04126 ancillary file (2019-11-29)
Supplement: Supplementary file 1 [file programdocumentation.pdf]

# Typical entanglement for Gaussian states: Program code for computing moments

Motohisa Fukuda and Robert K 旦 nig

March 11, 2019

In this document, we briefly describe the programs used to compute the moments listed in appendix $C$ of our paper. We give both MATHEMATICA and python code. They rely on the RTNI package [1] for taking averages over the unitary group.

## 1 MATHEMATICA computation of moments

### 1.1 Installation

The code for the RTNI package is available at the RTNI Github repository. The MATHEMATICA programs of RTNI (as well as precomputed Weingarten functions) should be placed in the same folder as the notebook "CovarianceMatrixMoments_using_RTNI.nb"

### 1.2 Formulas used in the MATHEMATICA program

Following the notations introduced in Section 2 of the main paper, we use the following expressions for the second and fourth moments:

**Lemma 1.1.** *We have*

$$\mathrm{Tr}((JM_{n,k})^2) = \mathrm{Tr}((JR)^2) \tag{1}$$

$$\mathrm{Tr}((JM_{n,k})^4) = \mathrm{Tr}((JR)^4) \tag{2}$$

*where $R$ is a $2n \times 2n$ matrix such that*

$$JR = \begin{pmatrix} -i\Pi\overline{U}BU^T & -\Pi\overline{U}A\overline{U}^T \\ -\Pi UAU^T & i\Pi UB\overline{U}^T \end{pmatrix} . \tag{3}$$

*Proof.* We can write

$$S = F \begin{pmatrix} U & 0 \\ 0 & \overline{U} \end{pmatrix} F^{-1} \qquad \text{where} \qquad F = \frac{1}{\sqrt{2}} \begin{pmatrix} I & iI \\ iI & I \end{pmatrix} \tag{4}$$

Also,

$$F^{-1}\hat{Z}_n(F^{-1})^T = \frac{1}{2} \begin{pmatrix} A & -iB \\ -iB & -A \end{pmatrix} , \tag{5}$$

hence

$$M_n = F \begin{pmatrix} U & 0 \\ 0 & \overline{U} \end{pmatrix} \frac{1}{2} \begin{pmatrix} A & -iB \\ -iB & -A \end{pmatrix} \begin{pmatrix} U^T & 0 \\ 0 & \overline{U}^T \end{pmatrix} F^T \tag{6}$$

$$= F \begin{pmatrix} UAU^T & -iUB\overline{U}^T \\ -i\overline{U}BU^T & -\overline{U}A\overline{U}^T \end{pmatrix} F^T \ . \tag{7}$$

Since $\hat{\Pi}$ commutes with $J$ and $F$, we obtain

$$\begin{aligned} M_{n,k} &= \hat{\Pi} M_n \\ &= FRF^T \qquad \text{where} \qquad R = \begin{pmatrix} \Pi UAU^T & -i\Pi UB\overline{U}^T \\ -i\Pi\overline{U}BU^T & -\Pi\overline{U}A\overline{U}^T \ . \end{pmatrix} \end{aligned} \tag{8}$$

Since $F^T JF = J$, we obtain

$$\mathrm{Tr}(JM_{n,k})^2 = \mathrm{Tr}(JFRF^TJFRF^T) = \mathrm{Tr}(JRJR) \tag{9}$$

$$\mathrm{Tr}(JM_{n,k})^4 = \mathrm{Tr}(JR)^4 \ . \tag{10}$$

□

### 1.3 Mathematica computation and processing of moments

The MATHEMATICA program uses expressions (1) and (2) to compute the moments of interest. It proceeds as follows:

1. It symbolically computes powers of $JR$ by implementing two-by-two-matrix multiplication for block-matrices whose entries are multinomial expressions involving products of the matrices $\{\Pi, U, \overline{U}, U^T, \overline{U}^T = U^*\}$.
2. It then invokes the routine MultinomialexpectationvalueHaar of the RTNI package to compute the corresponding expectation value for each entry of $JR$.
3. Various substitution rules (related to the cyclicity of the trace and identities such as $\mathrm{Tr}(A^T) = \mathrm{Tr}(A)$, as well as the fact that $\mathrm{Tr}(\Pi) = k$) are used to simplify the expressions.
4. Substitution rules related to the asymptotic behavior are applied (corresponding to the leading order in the middle column in the tables in Appendix C).

Additional documentation is provided in the program.

## 2 python computation of moments

### 2.1 Installation

The python programs of RTNI are available on the RTNI Github repository. They should be placed within the same folder as the programs "GaussianState_Pipeline.py" and "GS_source.py" provided with the current paper.

### 2.2 python computation and processing of moments

In the file "GaussianState_Pipeline.py", one can find two pipelines which calculate the second and fourth moments. These compute the average of the following polynomials of matrices. Let $G = \Pi U A U^*$ and $H = -i\Pi U B U^*$ such that

$$\mathbb{E}\,\mathrm{Tr}\left[(JM)^2\right] = \mathbb{E}\,\mathrm{Tr}\left[\begin{pmatrix}\bar{H} & \bar{G}\\ G & H\end{pmatrix}^2\right] = \mathbb{E}\,\mathrm{Tr}\left[\bar{H}^2 + \bar{G}G + G\bar{G} + H^2\right] = \mathbb{E}\,\mathrm{Tr}\left[2H^2 + 2G\bar{G}\right]. \tag{11}$$

and

$$\mathbb{E}\,\mathrm{Tr}(JM)^4 = \mathbb{E}\,\mathrm{Tr}\left[\begin{pmatrix}\bar{H} & \bar{G}\\ G & H\end{pmatrix}^4\right] = \mathbb{E}\,\mathrm{Tr}\left[H^4 + \bar{H}^4 + 2(G\bar{G})^2 + 4\bar{H}^2\bar{G}G + 4\bar{H}\bar{G}HG + 4H^2G\bar{G}\right] \tag{12}$$

$$= \mathbb{E}\,\mathrm{Tr}\left[2H^4 + 2(G\bar{G})^2 + 8G\bar{G}H^2 + 4G\bar{H}\bar{G}H\right]. \tag{13}$$

Here, we used the fact that $\mathbb{E}\,\mathrm{Tr}\,H^4 = \mathbb{E}\,\mathrm{Tr}\,\bar{H}^4$ and $\mathbb{E}\,\mathrm{Tr}[\bar{H}^2\bar{G}G] = \mathbb{E}\,\mathrm{Tr}[H^2G\bar{G}]$, because the non-random matrices appearing in the definition of $G$ and $H$ are real.

The above expressions are used to encode the second and fourth moments in terms $(e_i, w_i)$ for $i = 1, 2$ and $(E_i, W_i)$ for $i = 1, 2, 3, 4$, respectively, in the program. For example, the term $2H^2$ in (11) is represented by

```
e1 = ['P','U','B','U*','P','U','B','U*']
w1 = -2
```

These variables are the inputs into the pipelines. They are transformed by the function "Translator" into the format used by the RTNI package.

The outputs will be "average" and "Average" for the second and forth moments, respectively. The function "FinalTable" tidies them up and produces tables as in Appendix C. They are written as nested lists, where each element corresponds to each line of tables.

Consider for example the case of the second moment. Here is the first element of the nested list of the output:

```
[[['A', 'A']], 2*k*(k + 1)/(n*(n + 1)), [2*K**2, 2*kappa - 2],
[C*lam, zeta + 1], [2*C*K**2*lam, 2*kappa + zeta - 1]]
```

This means that the coefficient of $\mathrm{Tr}[A^2]$ is $2k(k+1)/(n(n+1))$, its leading term in the coefficient is $2K^2n^{2\kappa-2}$ and the asymptotic bound for $\mathrm{Tr}[A^2]$ is $C\lambda n^{\zeta+1}$ so that as a whole this term behaves asymptotically as $2CK^2\lambda n^{2\kappa+\zeta-1}$. The nested structure for matrices represents how the trace is applied, for another example, [['B'], ['B']] means $(\mathrm{Tr}\,B)^2$.

# References


[1] *Motohisa Fukuda, Robert Koenig and Ion Nechita* RTNI — A symbolic integrator for Haar-random tensor networks. arXiv:1902.08539. January 2019.
